# Supplementary material for: Simplification of the Fermi-L\"owdin Self-Interaction Correction Method for Efficient Self-Interaction-Free Density Functional Calculations
Source: arXiv:2308.04664 source file (2025-08-06)
Supplement: Supplementary file 1 [file SI.pdf]

# Supplementary information for: “Complexity reduction in self-interaction-free density functional calculations using the Fermi-Löwdin self-interaction correction method"

Selim Romero,[1] Yoh Yamamoto,[2] Tunna Baruah,[2] and Rajendra R. Zope[2]

[1]) *Computational Science Program,The University of Texas at El Paso, El Paso, Texas 79968*

[2]) *Department of Physics, University of Texas at El Paso,TX, 79968*

(Dated: 9 August 2023)

## S1. SUPPLEMENTARY DATA FOR THE vSOSIC CALCULATIONS

- The nuclear geometries and FOD coordinates used in this work can be found at `https://github.com/FLOSIC/si_vSOSIC`.
- Fig. S1 compares the PZSIC and vSOSIC eigenvalue spectra for LiBr and NaBr.
- Table S1 shows vSOSIC total energy of atoms.
- Table S2 shows the average polarizability of six molecules. The polarizability tensor $\alpha_{ij}$ is calculated by taking the derivative of the dipole moments $\vec{\mu}$ with respect to an applied electric field components $F_j$ using finite difference method as:

$$\alpha_{ij} = \left.\frac{\partial \mu_i}{\partial F_j}\right|_{F_j=0} = \lim_{F_j \to 0} \frac{\mu_i(F_j) - \mu_i(-F_j)}{2F_j}. \tag{S1}$$

  The electric field strength of 0.005 a.u. is used. The average polarizability $\alpha_{avg} = (\alpha_{11} + \alpha_{22} + \alpha_{33})/3$ is calculated from the trace of the polarizability tensor.

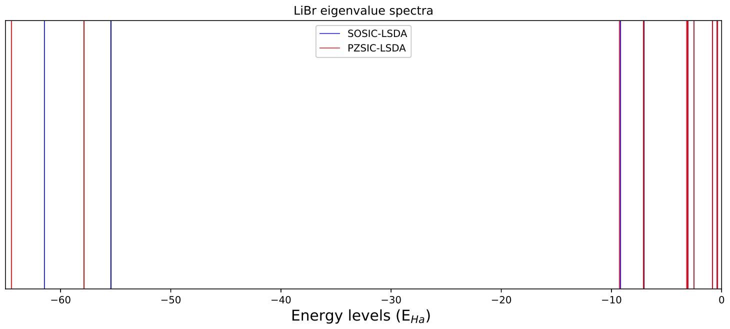


(a)

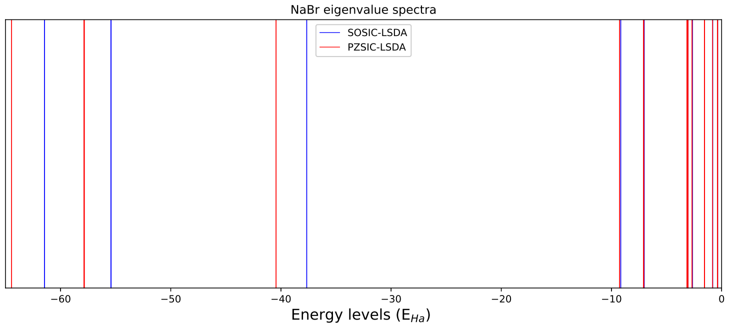


(b)

FIG. S1: Eigenvalue energy spectra for (a) LiBr and (b) NaBr systems with small core removed from the SIC calculation. The 1s eigenenergies are removed for clarity. Note the agreement between the two sets for valence eigenvalues.

TABLE S1: Mean absolute error (MAE) in $E_h$ for the total energy of an atom from hydrogen to argon compared against the values from reference 1.

| Functional | Method | MAE($E_h$) |
|---|---|---|
| LSDA | DFA | 0.726 |
| LSDA | PZSIC | 0.379 |
| LSDA | vSOSIC | 0.607 |
| PBE | DFA | 0.083 |
| PBE | PZSIC | 0.158 |
| PBE | vSOSIC | 0.199 |
| $r^2$SCAN | DFA | 0.011 |
| $r^2$SCAN | PZSIC | 0.172 |
| $r^2$SCAN | vSOSIC | 0.085 |

TABLE S2: The average polarizability (in $a_0^3$) of a set of six molecules.

| System | Functional | DFA | PZSIC | vSOSIC | Exp [a] |
|---|---|---|---|---|---|
| $AsH_3$ | LSDA | 37.4 | 32.4 | 32.7 | 36.90 |
| | PBE | 34.5 | 33.2 | 33.9 | |
| | r$^2$SCAN | 35.7 | 33.6 | 33.7 | |
| $AsCl_3$ | LSDA | 78.4 | 68.6 | 69.3 | 76.73 |
| | PBE | 78.0 | 71.8 | 70.7 | |
| | r$^2$SCAN | 75.6 | 70.5 | 72.0 | |
| $As_4$ | LSDA | 117.0 | 111.0 | 109.4 | 116.70 |
| | PBE | 118.0 | 117.8 | 110.2 | |
| | r$^2$SCAN | 114.7 | 110.9 | 113.3 | |
| $GeCl_4$ | LSDA | 88.6 | 73.9 | 76.6 | 84.29 |
| | PBE | 87.6 | 81.9 | 78.4 | |
| | r$^2$SCAN | 84.5 | 79.0 | 79.8 | |
| $GeF_4$ | LSDA | 29.6 | 23.8 | 23.3 | 27.33 |
| | PBE | 29.5 | 24.4 | 23.7 | |
| | r$^2$SCAN | 27.8 | 23.0 | 23.4 | |
| $GeH_4$ | LSDA | 37.5 | 30.1 | 32.9 | 32.19 |
| | PBE | 36.6 | 32.4 | 34.4 | |
| | r$^2$SCAN | 35.4 | 32.8 | 33.1 | |
| Benzene | LSDA | 70.5 | 67.1 | 68.4 | 67.79 |
| | PBE | 70.2 | 68.3 | 69.2 | |
| | r$^2$SCAN | 69.6 | 70.4 | 68.0 | |
| MAE (MSE) | LSDA | 2.4 (2.4) | 5.0 (-5.0) | 4.6 (-4.2) | |
| | PBE | 2.5 (1.8) | 2.3 (-1.7) | 4.1 (-3.1) | |
| | r$^2$SCAN | 1.5 (0.2) | 4.0 (-3.1) | 3.0 (-2.7) | |

[a] Reference 2

## S2. PZSIC-r$^2$SCAN PERFORMANCE AND INTEGRATION MESH DEPENDENCE

We compared the performance and mesh dependence of PZSIC-r$^2$SCAN on the total energies of atoms, atomization energies, barrier heights, and cluster binding energy of water molecules. For this purpose, we have prepared four mesh settings that differ by fineness in their integration grids as follows,

- `medium` - A default NRLMOL mesh for FLOSIC calculation. On average, it has 25000 grid points per atom. This results in the integration of charge density that is accurate to the order of $10^{-8}$e.
- `fine` - Fine mesh approximately 1.3 times more grid points than the default mesh.
- `vfine` - Very fine mesh approximately 1.6 times more grid points than the default mesh.
- `sfine` - Super fine mesh approximately 4.6-5.6 times more grid points than the default mesh. Approximately 140000 grid points per atom. This mesh allows accurate numerical integration with SCAN.

With these mesh settings, we have obtained the results as shown in Table S3-S9. We find that For PZSIC-r$^2$SCAN functional, the mesh setting affects the total energies of atoms and molecules in order of $10^{-4}E_\mathrm{h}$. In the atom total energies, mean absolute errors (MAE) of PZSIC-r$^2$SCAN (MAE = 0.172 $E_\mathrm{h}$) is slightly larger than PZSIC-SCAN (0.147 $E_\mathrm{h}$) and PZSIC-rSCAN (0.140 $E_\mathrm{h}$). For the electron affinity (EA) of atoms, PZSIC-r$^2$SCAN performance is the same as PZSIC-SCAN with MAE, 0.36 eV for 12 EAs and 0.34 eV for 20 EAs, which are in agreement up to second decimal places in MAEs. PZSIC-rSCAN MAEs are approximately 0.03 eV smaller than PZSIC-SCAN and PZSIC-r$^2$SCAN. For the ionization potential (IP) of atoms, PZSIC-r$^2$SCAN performs similarly to PZSIC-rSCAN (MAE = 0.34 eV) for the set of 35 atoms. The atomization energy performance of PZSIC-r$^2$SCAN (MAE = 26.2 kcal/mol) is close to PZSIC-SCAN (MAE = 26.5 kcal/mol). The performance in the barrier heights using the BH6 set remains the same for PZSIC-SCAN, PZSIC-rSCAN, and PZSIC-r$^2$SCAN where their discrepancies are within 0.2 kcal/mol among the three functionals.

From the above observation, we conclude that for energetic performance, r$^2$SCAN provides the identical performance with `medium` and with `sfine` mesh settings. In the energy landscape of covalent bond stretching, we observed the need to use mesh denser than the `medium` to accurately describe it. Sufficient grid points are needed for the "kinks"

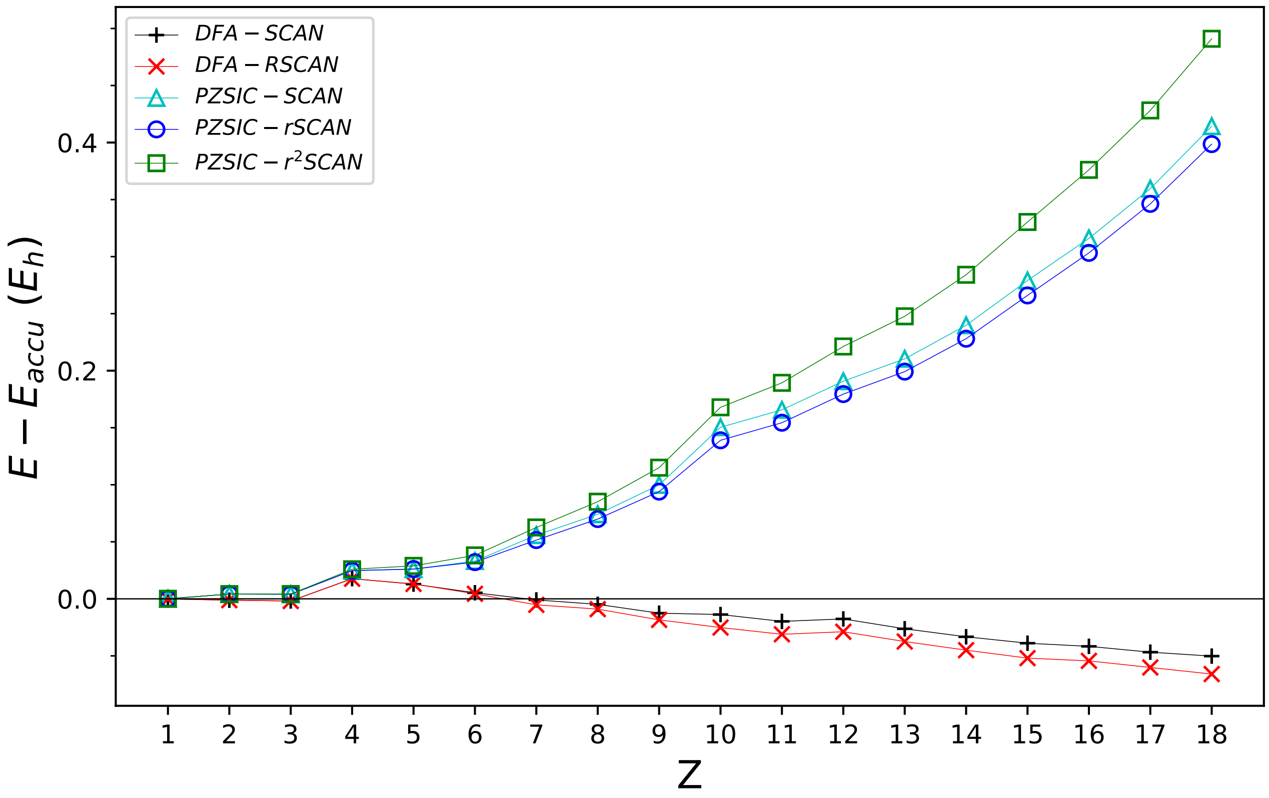


FIG. S2: Energy difference (in $E_{\mathrm{h}}$) between the total energy of atoms and the values from Ref. 1. The `fine` mesh setting was used.

that appear in the meta-GGA XC potential curve to integrate energy density accurately. We have tuned the radial grid point density in the FLOSIC code for providing accurate charge density integrations for the PZSIC-r$^2$SCAN functional.

TABLE S3: The total energy of atoms hydrogen to argon in ($E_h$) using PZSIC-r$^2$SCAN functional and varying mesh configurations.

| $Z$ | medium | fine | vfine | sfine | Ref. 1 |
|---|---|---|---|---|---|
| 1 | -0.49992 | -0.49992 | -0.49992 | -0.49992 | -0.500 |
| 2 | -2.89954 | -2.89954 | -2.89954 | -2.89954 | -2.904 |
| 3 | -7.47386 | -7.47377 | -7.47376 | -7.47376 | -7.478 |
| 4 | -14.64144 | -14.64144 | -14.64148 | -14.64146 | -14.667 |
| 5 | -24.62500 | -24.62492 | -24.62494 | -24.62493 | -24.654 |
| 6 | -37.80689 | -37.80689 | -37.80685 | -37.80681 | -37.845 |
| 7 | -54.52662 | -54.52684 | -54.52671 | -54.52669 | -54.589 |
| 8 | -74.98216 | -74.98215 | -74.98222 | -74.98220 | -75.067 |
| 9 | -99.61892 | -99.61899 | -99.61893 | -99.61893 | -99.734 |
| 10 | -128.76969 | -128.76967 | -128.76971 | -128.76968 | -128.938 |
| 11 | -162.06525 | -162.06514 | -162.06521 | -162.06518 | -162.255 |
| 12 | -199.83177 | -199.83173 | -199.83178 | -199.83178 | -200.053 |
| 13 | -242.09831 | -242.09840 | -242.09836 | -242.09837 | -242.346 |
| 14 | -289.07492 | -289.07486 | -289.07485 | -289.07490 | -289.359 |
| 15 | -340.92864 | -340.92844 | -340.92844 | -340.92847 | -341.259 |
| 16 | -397.73395 | -397.73414 | -397.73402 | -397.73408 | -398.110 |
| 17 | -459.71982 | -459.72006 | -459.71998 | -459.72001 | -460.148 |
| 18 | -527.04902 | -527.04939 | -527.04931 | -527.04945 | -527.540 |
| MAE | 0.172 | 0.172 | 0.172 | 0.172 | |

TABLE S4: Mean absolute errors (MAE) in $E_h$ for the total energy of atoms from hydrogen to argon using the SCAN family of functionals and several mesh configurations. The MAEs are computed with respect to the theoretical estimates in Ref. 1.

| Method | Mesh | MAE ($E_h$) |
|---|---|---|
| SCAN | `sfine` | 0.019 |
| rSCAN | `sfine` | 0.027 |
| $r^2$SCAN | `sfine` | 0.010 |
| PZSIC-SCAN | `sfine` | 0.147 |
| PZSIC-rSCAN | `sfine` | 0.140 |
| PZSIC-$r^2$SCAN | `medium` | 0.172 |
| PZSIC-$r^2$SCAN | `fine` | 0.172 |
| PZSIC-$r^2$SCAN | `vfine` | 0.172 |
| PZSIC-$r^2$SCAN | `sfine` | 0.172 |

TABLE S5: Mean absolute error (in eV) in electron affinity obtained with ΔSCF with respect to the experiment reported in Ref. 2. Here 12 EAs refer to EAs of H, Li B, C, O, F, Na, Al, Si, P, S, and Cl atoms. 20 EAs include K, Ti, Cu, Ga, Ge, As, Se, and Br atoms in addition to 12 EAs.

| Method | Mesh | 12 EAs | 20 EAs |
|---|---|---|---|
| PZSIC-SCAN | `sfine` | 0.364 | 0.341 |
| PZSIC-rSCAN | `sfine` | 0.329 | 0.314 |
| PZSIC-$r^2$SCAN | `medium` | 0.357 | 0.337 |
| PZSIC-$r^2$SCAN | `sfine` | 0.356 | 0.337 |

TABLE S6: Mean absolute error (in eV) in ionization potential obtained with ΔSCF with respect to the experiment reported in Ref. 2.

| Method | Mesh | Z=2-18 | Z=2-36 |
|---|---|---|---|
| PZSIC-SCAN | `sfine` | 0.274 | 0.259 |
| PZSIC-rSCAN | `sfine` | 0.222 | 0.342 |
| PZSIC-r$^2$SCAN | `medium` | 0.243 | 0.343 |
| PZSIC-r$^2$SCAN | `sfine` | 0.242 | 0.342 |

TABLE S7: Mean absolute error (in kcal/mol) for the atomization energies of the AE6 set.

| Method | Mesh | MAE (kcal/mol) |
|---|---|---|
| SCAN | `sfine` | 2.85 |
| rSCAN | `sfine` | 6.28 |
| r$^2$SCAN | `sfine` | 2.84 |
| PZSIC-SCAN | `sfine` | 26.52 |
| PZSIC-rSCAN | `sfine` | 21.63 |
| PZSIC-r$^2$SCAN | `medium` | 26.27 |
| PZSIC-r$^2$SCAN | `fine` | 26.33 |
| PZSIC-r$^2$SCAN | `vfine` | 26.28 |
| PZSIC-r$^2$SCAN | `sfine` | 26.24 |

TABLE S8: The mean absolute errors (MAE) in kcal/mol for the reaction barrier height of the BH6 set.

| Method | Mesh | MAE (kcal/mol) |
|---|---|---|
| SCAN | `sfine` | 7.86 |
| rSCAN | `sfine` | 9.41 |
| $r^2$SCAN | `sfine` | 7.55 |
| PZSIC-SCAN | `sfine` | 2.96 |
| PZSIC-rSCAN | `sfine` | 2.72 |
| PZSIC-$r^2$SCAN | `medium` | 2.78 |
| PZSIC-$r^2$SCAN | `fine` | 2.79 |
| PZSIC-$r^2$SCAN | `vfine` | 2.80 |
| PZSIC-$r^2$SCAN | `sfine` | 2.80 |

TABLE S9: Binding energy per molecule (in meV per $H_2O$) of water clusters from dimer to hexamers. The `medium` mesh setting was used.

| Cluster | SCAN | rSCAN | $r^2$SCAN | PZSIC-SCAN | PZSIC-rSCAN | PZSIC-$r^2$SCAN | CCSD(T)* |
|---|---|---|---|---|---|---|---|
| $(H_2O)_2$ | -118.0 | -118.2 | -112.6 | -110.2 | -110.7 | -105.3 | -108.6 |
| $(H_2O)_3$ | -256.7 | -256.6 | -244.3 | -232.1 | -231.2 | -220.5 | -228.4 |
| $(H_2O)_4$ | -334.3 | -336.7 | -321.0 | -301.1 | -302.7 | -287.4 | -297 |
| $(H_2O)_5$ | -350.8 | -351.9 | -335.5 | -317.3 | -318.0 | -301.9 | -311.4 |
| $(H_2O)_6$ B | -369.0 | -369.6 | -352.2 | -333.1 | -333.5 | -316.5 | -332.4 |
| $(H_2O)_6$ C | -373.2 | -373.4 | -355.6 | -336.3 | -340.8 | -324.5 | -330.5 |
| $(H_2O)_6$ P | -374.8 | -374.6 | -356.7 | -338.4 | -337.9 | -320.7 | -327.3 |
| $(H_2O)_6$ R | -359.5 | -360.4 | -343.8 | -326.3 | -326.7 | -310.5 | -320.1 |
| MAE | 35.1 | 35.7 | 20.8 | 4.9 | 5.7 | 8.6 | |

*Reference 3

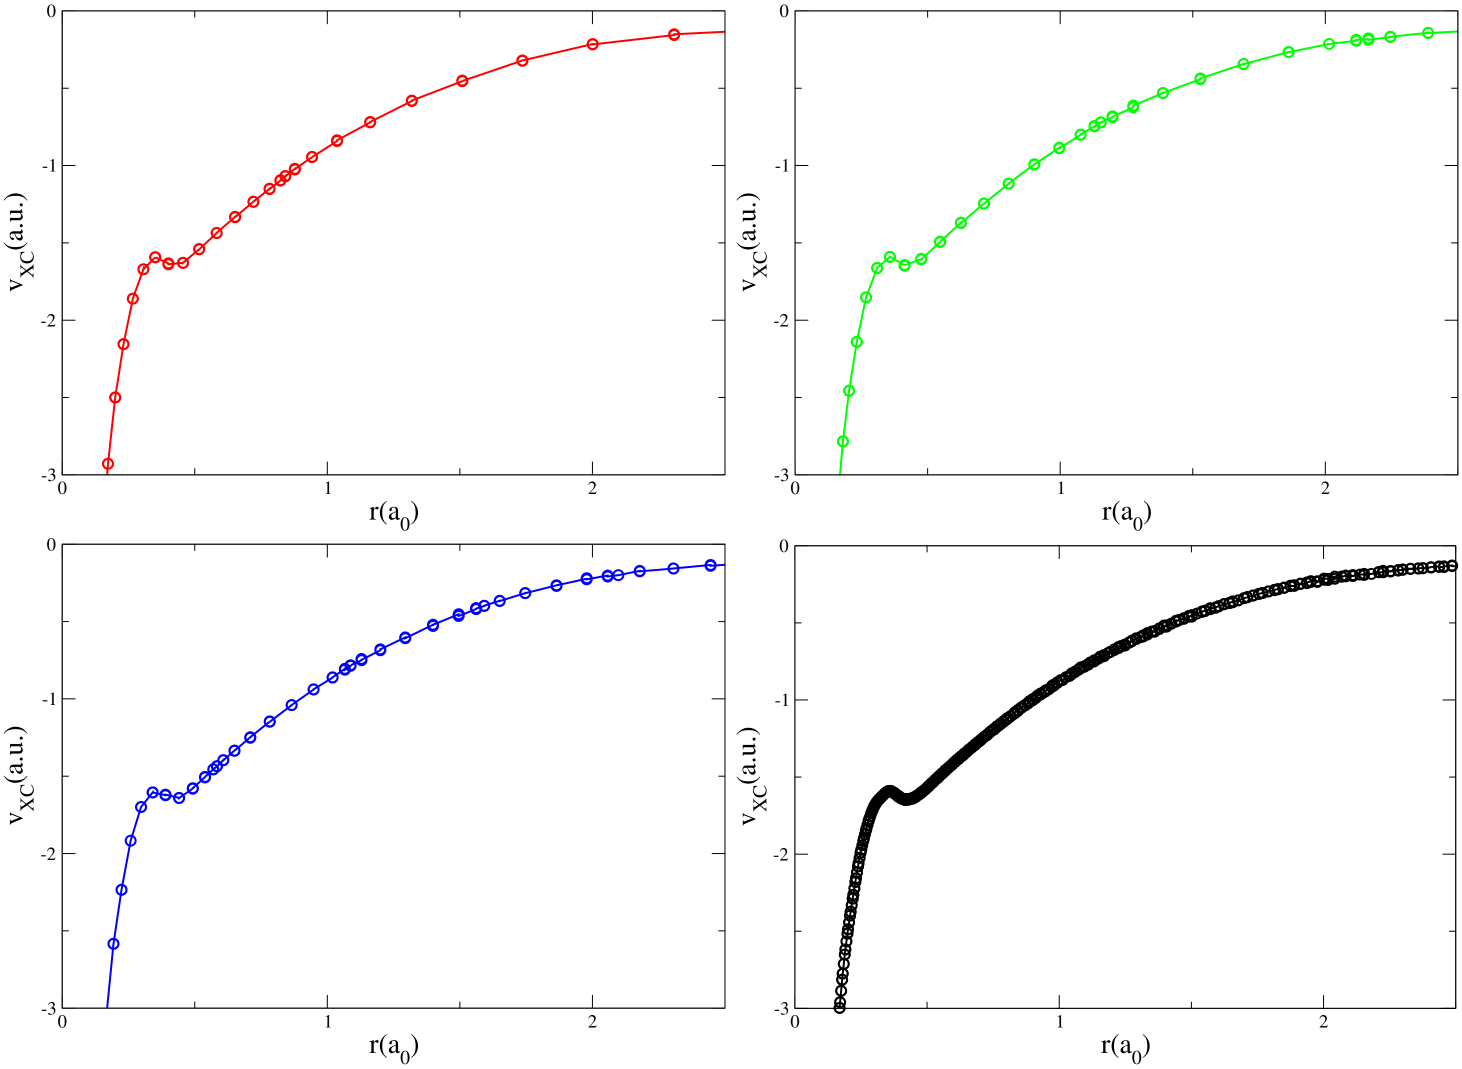


FIG. S3: $v_{XC}$ curves of neon atom from SIC-r$^2$SCAN calculations. The mesh settings used are (top left) medium, (top right) fine, (bottom left) vfine, and (bottom right) sfine. Data points indicate generated grid points.

## REFERENCES

[1]S. J. Chakravorty, S. R. Gwaltney, E. R. Davidson, F. A. Parpia, and C. F. p Fischer, “Ground-state correlation energies for atomic ions with 3 to 18 electrons,” Phys. Rev. A **47**, 3649–3670 (1993).

[2]National Institute of Standards and Technology, NIST Computational Chemistry Comparison and Benchmark Database NIST Standard Reference Database Number 101 Release 19, April 2018, Editor: Russell D. Johnson III `http://cccbdb.nist.gov/` DOI:10.18434/T47C7Z.

[3]D. Manna, M. K. Kesharwani, N. Sylvetsky, and J. M. L. Martin, “Conventional and explicitly correlated ab initio benchmark study on water clusters: Revision of the BEGDB and WATER27 data sets,” J. Chem. Theory Comput. **13**, 3136–3152 (2017), pMID: 28530805, https://doi.org/10.1021/acs.jctc.6b01046.
